# Supplementary material for: Revisiting Optimal Resilience of Fast Byzantine Consensus (Extended Version)
Source: arXiv:2102.12825 source file (2021-07-27)
Supplement: Supplementary file 1 [file appendix.tex]

\section{The Lower Bound Discrepancy} \label{app:mistake}

% \yan{[entire section is new, so I'm killing the color]}

As stated, our proof for the lower bound in Theorem~\ref{the:lower-bound} is very similar to that of Theorem \cite[Theorem V.1]{fab-paxos}. We now carefully contrast our works.
First, \cite{fab-paxos} defines a \emph{$(t,2)$-step consensus protocol} as a protocol which can tolerate $f$ Byzantine failures and satisfies the following: for every initial configuration $I$ and every set $F$ of at most $t$ processes ($t \leq f$), there
exists a \emph{two-step execution} (all correct processes learn by the end of the second round) from $I$ that is \emph{$F$-silent} (processes in $F$ do not take any actions). Then they conclude:

\begin{theorem}[Theorem V.1, \cite{fab-paxos}, paraphrased]
\label{thm:old-lower-bound}
Any $(t,2)$-step Byzantine fault-tolerant
consensus protocol requires at least $3f+2t+1$ processes.
\end{theorem}
 
Some remarks:
\begin{enumerate}
    \item Their definition of \emph{$(t,2)$-step Byzantine fault-tolerant} protocol is very strong; it actually includes no ``leader-based'' protocols, including their own main protocol in \cite{fab-paxos}. If the leader chosen by the initial configuration is faulty, then there cannot exist a two-step execution -- in particular, the processes must necessarily wait for the view-change algorithm.
    
    \item The point of the $\Suspects$ in our definition of \emph{two-step consensus protocol} is to protect against this scenario by limiting the suspects of fast two-step executions to processes other than the leader (or leaders). 
    % \todoA{What is ``$s$''?}. 
    % \yan{[the construction ``leader(s)'' means ``usually there is a single leader, but we could have multiple leaders in unusual situations''; it is an English construction and not a math construction. Since it might be confusing, we can just do ``leader'' too]} 
    This definition then actually applies to the protocols we discuss, including both our own and that of~\cite{fab-paxos}. 
    
 %   \item The point of our definition of \emph{influential process} is to ``capture'' the leader in these types of protocols without having to define ``leader'' as a special role. This definition allows us to treat the leader differently (in our proof, the influential process $p$).
    %
%    \todoA{I added my version below. I wanted to make it clearer that our goal was to make the proof as general as possible instead of focusing on a specific class of PBFT-like leader-based protocols.}
    
    \item The point of our definition of \emph{influential process} is to prove that every two-step consensus protocol has to have a ``leader'' in some sense.
    % This allows us to avoid restricting .
    It allows us to treat the ``leader'' (in our proof, the influential process $p$) differently from other processes
    without restricting the applicability of our lower bound to protocols that have structure similar to our protocol. 
    %\yan{[I trust your intuition over mine, so let's just use ``that'']}
    
    \item In~\cite{fab-paxos}'s proof of the lower bound, they have $5$ groups of sizes $(t, f, f, f, t)$, whereas we have $6$ groups of sizes $(1, t, f-1, f-1, f-1, t)$, with the isolated influential process $p$ forcing us to change the size-$f$ groups to $(f-1)$ for the hypothetical executions when $p$ is byzantine. This creates a total ``discount'' of $2$ processes, which explains our lower bound changing from $3f+2t+1$ to $3f+2t-1$.
    %
    %\todoA{The issue with the word ``allowing'' in this context is that it sounds a bit like we have the choice of making the group sizes larger, but this would contradict our upper bound (a.k.a.\ algorithm).}
\end{enumerate}
